# Supplementary material for: All in One: Exploring Unified Video-Language Pre-training
Source: arXiv:2203.07303 source file (2022-03-14)
Supplement: Supplementary file 1 [file model_scalability_table.tex]

\newcolumntype{g}{>{\columncolor{Gray}}c}
\begin{table}[h]
\footnotesize
\centering
\scalebox{\GlobalTableRescale}{
\begin{tabular}{@{}ll|rrr|rr}
Method & Params &Pre-training Time & \multicolumn{2}{c|}{Pretrain}  \\
 &  & & VTM& MLM  \\
\shline
TimeSformer&180.5M&\textcolor{darkergreen}{\checkmark}   \\
\end{tabular}
}
\caption{
\textbf{Different Model}.
}
\label{tab:abl_temporal_attn}
\end{table}
